# Supplementary material for: Applications of QR-based Vector-Valued Rational Approximation
Source: arXiv:2601.23237 source file (2026-11-13)
Supplement: Supplementary file 1 [file quad_sing_supp_exact_int.tex]

1e-08
1
0.0021526
0.90328
0.12074
0.98392
1.3901e-06
0.68039
3.1091e-05
0.37217
0.95405
0.01879
0.81051
0.00029576
7.1969e-08
0.2296
0.55002
0.99448
3.7276e-06
0.0068486
0.8637
1.3895e-07
0.054593
8.1562e-05
0.74511
1.3895e-08
0.93406
0.29785
7.5574e-06
0.00069196
0.47065
7.1969e-07
0.97194
0.03325
2.6827e-08
0.62083
0.08587
0.00015591
0.0042528
0.83775
5.1795e-07
0.17447
1.3626e-05
0.99805
3.7276e-08
0.42381
0.011682
