# Supplementary material for: Applications of QR-based Vector-Valued Rational Approximation
Source: arXiv:2601.23237 source file (2026-11-13)
Supplement: Supplementary file 2 [file quad_supp_exact_int.tex]

1
0.00054058
0.093872
0.93146
0.74818
3.7276e-08
0.0093978
0.98483
0.44809
1.3895e-06
0.84835
1.6686e-05
0.23085
0.61751
8.3034e-05
1e-08
0.0031956
0.96406
0.039654
0.33519
1.9307e-07
0.89174
3.5545e-06
0.15142
0.00022747
0.69123
0.020213
1.3895e-08
0.52999
3.7276e-07
0.9951
0.001238
7.1969e-06
0.80214
0.062478
3.5643e-05
5.1795e-08
0.388
0.0055824
0.94858
7.1969e-07
0.18966
7.1969e-08
0.00015017
